# Supplementary material for: Finite-Temperature Toroidal Moment Amenable to Direct Observation in an Fe$_{10}$Dy$_{10}$ Molecular Ring
Source: arXiv:2509.05424 source file (2026-05-23)
Supplement: Supplementary file 1 [file GiantToroidal_SuppInfo.pdf]

# Supplementary Information: Giant Molecular Toroidal Moment Amenable to Direct Observation in a Fe<sub>10</sub>Dy<sub>10</sub> Ring

Alessandro Soncini<sup>1\*</sup>, Kieran Hymas<sup>2</sup>, Jonas Braun<sup>3,4,5</sup>,  
Yannik F. Schneider<sup>3</sup>, Simone Calvello<sup>1</sup>, Amer Baniodeh<sup>3</sup>,  
Yanhua Lan<sup>3</sup>, Wolfgang Wernsdorfer<sup>5,6</sup>, Marco Affronte<sup>7</sup>,  
Christopher E. Anson<sup>3</sup>, Annie K. Powell<sup>3,4,5\*</sup>

<sup>1\*</sup>Department of Chemical Sciences, University of Padova, Via Marzolo  
1, Padova, 35123, Italy.

<sup>2</sup>Commonwealth Scientific and Industrial Research Organisation,  
CSIRO, Clayton, 3168, Victoria, Australia.

<sup>3</sup>Institute of Inorganic Chemistry, Karlsruhe Institute of Technology  
(KIT), Kaiserstr. 12, Karlsruhe, 76131, Germany.

<sup>4</sup>Institute of Nanotechnology, Karlsruhe Institute of Technology (KIT),  
Kaiserstr. 12, Karlsruhe, 76131, Germany.

<sup>5</sup>Institute for Quantum Materials and Technologies, Karlsruhe Institute  
of Technology (KIT), Kaiserstr. 12, Karlsruhe, 76131, Germany.

<sup>6</sup>Physikalisches Institut, Karlsruhe Institute of Technology (KIT),  
Kaiserstr. 12, Karlsruhe, 76131, Germany.

<sup>7</sup>Dipartimento di Scienze Fisiche, Informatiche e Matematiche,  
University of Modena and Reggio Emilia, Via Campi 213A, Modena,  
41125, Italy.

\*Corresponding author(s). E-mail(s): [alessandro.soncini@unipd.it](mailto:alessandro.soncini@unipd.it);  
[annie.powell@kit.edu](mailto:annie.powell@kit.edu);

## Contents

|          |                                                             |           |
|----------|-------------------------------------------------------------|-----------|
| <b>1</b> | <b>Supplementary Note 1: Computational Data</b>             | <b>3</b>  |
| <b>2</b> | <b>Supplementary Note 2: Toroidal and Magnetic Spectrum</b> | <b>13</b> |
| <b>3</b> | <b>Supplementary Note 3: Synthesis</b>                      | <b>14</b> |
| <b>4</b> | <b>Supplementary Note 4: AC SQUID Magnetometry</b>          | <b>15</b> |
| <b>5</b> | <b>Supplementary Note 5: MicroSQUID</b>                     | <b>16</b> |

# 1 Supplementary Note 1: Computational Data

As reported in the Methods section of the manuscript, subsection 5.1, we performed Configurationally Averaged Hartree Fock (CAHF)/Complete Active Space Configuration Interaction-Spin Orbit (CASCI-SO) calculations on the five symmetry unique  $[\text{Dy}^{\text{III}}\text{Fe}_2^{\text{III}}(\text{MeTeaH}^{2-})(\text{MeTea}^{3-})_2(\text{CH}_3\text{O}^-)_2\text{NO}_3^-]^{2-}$  (extended) fragments of the  $\text{Fe}_{10}\text{Dy}_{10}$  molecular wheel using the in-house developed *ab initio* quantum chemistry code CERES [1, 2], a methodology which allows for the full representation of the spin-orbit coupling problem in the complete basis of the 2002 states arising from full set of  $4f^9$  Russell-Saunders terms. In the following we report ten tables, two for each of the five fragments, reporting the obtained energy spectrum for the eight lowest lying Kramers Doublets (KD) describing the splitting of the ion's  $^6H_{15/2}$  ground spin-orbit multiplet and all the calculated  $g$ -tensors for each KD (Tables S1 to S5), and the Cartesian coordinates of the five fragments employed in the calculations (Tables S6 to S10).

**Table S1** Energy levels ( $E$  in  $\text{cm}^{-1}$ ),  $g$ -tensor principal values ( $g_X, g_Y, g_Z$ ), and magnetic axes  $\ell$  for Dy(III) centre 1. Lower-case  $x, y, z$  denote the molecular Cartesian frame; upper-case  $X, Y, Z$  denote the magnetic axes frame.

| Level | $E$ ( $\text{cm}^{-1}$ ) | $g_X$  | $g_Y$  | $g_Z$   | $\ell_X$ | $\ell_Y$ | $\ell_Z$ |   |
|-------|--------------------------|--------|--------|---------|----------|----------|----------|---|
| 1     | 0.0000                   | 0.0513 | 0.1079 | 19.5543 | 0.6606   | 0.0266   | -0.7503  | x |
|       |                          |        |        |         | 0.4621   | -0.8021  | 0.3784   | y |
|       |                          |        |        |         | 0.5917   | 0.5966   | 0.5422   | z |
| 2     | 104.9188                 | 1.4336 | 3.2376 | 15.1467 | -0.7489  | -0.4732  | -0.4640  | x |
|       |                          |        |        |         | -0.5313  | 0.8471   | -0.0064  | y |
|       |                          |        |        |         | -0.3961  | -0.2417  | 0.8858   | z |
| 3     | 159.3273                 | 0.0425 | 3.6814 | 13.2187 | -0.8349  | 0.5326   | -0.1385  | x |
|       |                          |        |        |         | 0.3661   | 0.7255   | 0.5827   | y |
|       |                          |        |        |         | 0.4109   | 0.4358   | -0.8008  | z |
| 4     | 245.9281                 | 2.6952 | 7.3032 | 9.0668  | 0.5825   | -0.7105  | 0.3948   | x |
|       |                          |        |        |         | -0.7508  | -0.2841  | 0.5964   | y |
|       |                          |        |        |         | 0.3116   | 0.6438   | 0.6989   | z |
| 5     | 350.8657                 | 1.6897 | 2.5212 | 12.9296 | 0.4253   | -0.1921  | -0.8844  | x |
|       |                          |        |        |         | 0.6376   | 0.7571   | 0.1422   | y |
|       |                          |        |        |         | -0.6423  | 0.6244   | -0.4445  | z |
| 6     | 430.7699                 | 0.4442 | 4.1951 | 12.8282 | 0.9705   | 0.0212   | 0.2401   | x |
|       |                          |        |        |         | -0.2100  | 0.5633   | 0.7991   | y |
|       |                          |        |        |         | -0.1183  | -0.8260  | 0.5512   | z |
| 7     | 471.1037                 | 1.4812 | 3.3161 | 13.7486 | -0.8044  | -0.4058  | -0.4339  | x |
|       |                          |        |        |         | 0.5840   | -0.6740  | -0.4524  | y |
|       |                          |        |        |         | 0.1089   | 0.6173   | -0.7792  | z |
| 8     | 508.6755                 | 0.4560 | 2.6369 | 16.7674 | 0.0956   | -0.6436  | -0.7594  | x |
|       |                          |        |        |         | -0.1087  | 0.7516   | -0.6507  | y |
|       |                          |        |        |         | 0.9895   | 0.1448   | 0.0019   | z |

**Table S2** Energy levels ( $E$  in  $\text{cm}^{-1}$ ),  $g$ -tensor principal values ( $g_X, g_Y, g_Z$ ), and magnetic axes  $\ell$  for Dy(III) centre 2. Lower-case  $x, y, z$  denote the molecular Cartesian frame; upper-case  $X, Y, Z$  denote the magnetic axes frame.

| Level | $E$ ( $\text{cm}^{-1}$ ) | $g_X$  | $g_Y$  | $g_Z$   | $\ell_X$ | $\ell_Y$ | $\ell_Z$ |   |
|-------|--------------------------|--------|--------|---------|----------|----------|----------|---|
| 1     | 0.0000                   | 0.0739 | 0.1696 | 19.3989 | -0.6751  | 0.7239   | -0.1423  | x |
|       |                          |        |        |         | 0.2088   | 0.3725   | 0.9042   | y |
|       |                          |        |        |         | 0.7076   | 0.5807   | -0.4026  | z |
| 2     | 109.9774                 | 1.6588 | 4.1751 | 14.0786 | 0.6252   | 0.7327   | -0.2688  | x |
|       |                          |        |        |         | -0.0877  | -0.2763  | -0.9571  | y |
|       |                          |        |        |         | -0.7755  | 0.6219   | -0.1085  | z |
| 3     | 156.9658                 | 1.8326 | 3.1368 | 12.6125 | 0.1309   | -0.8073  | -0.5755  | x |
|       |                          |        |        |         | -0.7464  | 0.3018   | -0.5931  | y |
|       |                          |        |        |         | 0.6525   | 0.5072   | -0.5631  | z |
| 4     | 243.9130                 | 1.6464 | 4.8045 | 11.0403 | -0.7540  | 0.5337   | -0.3831  | x |
|       |                          |        |        |         | -0.0561  | 0.5287   | 0.8469   | y |
|       |                          |        |        |         | -0.6545  | -0.6600  | 0.3687   | z |
| 5     | 305.3286                 | 2.5094 | 4.0827 | 11.8639 | -0.7852  | 0.6186   | -0.0297  | x |
|       |                          |        |        |         | -0.6172  | -0.7855  | -0.0453  | y |
|       |                          |        |        |         | -0.0513  | -0.0173  | 0.9985   | z |
| 6     | 372.1516                 | 1.0320 | 2.4707 | 16.0101 | 0.5362   | 0.6930   | -0.4820  | x |
|       |                          |        |        |         | -0.8427  | 0.4066   | -0.3529  | y |
|       |                          |        |        |         | -0.0486  | 0.5954   | 0.8020   | z |
| 7     | 434.6479                 | 0.1362 | 0.5869 | 18.1414 | 0.8994   | -0.3853  | -0.2066  | x |
|       |                          |        |        |         | -0.1727  | -0.7472  | 0.6418   | y |
|       |                          |        |        |         | 0.4016   | 0.5415   | 0.7385   | z |
| 8     | 485.3261                 | 0.3935 | 0.6378 | 18.5629 | 0.1299   | 0.2232   | -0.9661  | x |
|       |                          |        |        |         | -0.6000  | 0.7934   | 0.1026   | y |
|       |                          |        |        |         | 0.7894   | 0.5663   | 0.2369   | z |



**Table S3** Energy levels ( $E$  in  $\text{cm}^{-1}$ ),  $g$ -tensor principal values ( $g_X, g_Y, g_Z$ ), and magnetic axes  $\ell$  for Dy(III) centre 3. Lower-case  $x, y, z$  denote the molecular Cartesian frame; upper-case  $X, Y, Z$  denote the magnetic axes frame.

| Level | $E$ ( $\text{cm}^{-1}$ ) | $g_X$  | $g_Y$  | $g_Z$   | $\ell_X$ | $\ell_Y$ | $\ell_Z$ |   |
|-------|--------------------------|--------|--------|---------|----------|----------|----------|---|
| 1     | 0.0000                   | 0.1966 | 0.5761 | 19.0879 | 0.0571   | -0.4645  | -0.8837  | x |
|       |                          |        |        |         | -0.9976  | 0.0084   | -0.0688  | y |
|       |                          |        |        |         | 0.0394   | 0.8855   | -0.4629  | z |
| 2     | 60.2817                  | 1.3496 | 2.5570 | 16.1305 | -0.5151  | 0.8305   | -0.2118  | x |
|       |                          |        |        |         | -0.8547  | -0.5162  | 0.0547   | y |
|       |                          |        |        |         | -0.0639  | 0.2092   | 0.9758   | z |
| 3     | 107.5464                 | 0.3789 | 2.6666 | 13.5211 | -0.2560  | 0.2621   | -0.9305  | x |
|       |                          |        |        |         | -0.3631  | 0.8660   | 0.3438   | y |
|       |                          |        |        |         | 0.8959   | 0.4259   | -0.1266  | z |
| 4     | 168.0204                 | 3.0391 | 6.5057 | 10.2668 | 0.3005   | 0.8381   | -0.4553  | x |
|       |                          |        |        |         | 0.1280   | 0.4376   | 0.8900   | y |
|       |                          |        |        |         | 0.9452   | -0.3257  | 0.0242   | z |
| 5     | 243.0220                 | 1.6532 | 2.9395 | 12.8906 | -0.2935  | -0.9139  | -0.2805  | x |
|       |                          |        |        |         | -0.5064  | 0.3975   | -0.7652  | y |
|       |                          |        |        |         | 0.8108   | -0.0826  | -0.5795  | z |
| 6     | 316.5837                 | 1.4895 | 5.2113 | 11.3402 | -0.6522  | -0.7577  | 0.0218   | x |
|       |                          |        |        |         | 0.0562   | -0.0197  | 0.9982   | y |
|       |                          |        |        |         | -0.7560  | 0.6523   | 0.0554   | z |
| 7     | 340.2952                 | 1.7217 | 4.3676 | 14.1119 | 0.3201   | 0.8156   | -0.4820  | x |
|       |                          |        |        |         | -0.2629  | 0.5652   | 0.7819   | y |
|       |                          |        |        |         | 0.9102   | -0.1236  | 0.3954   | z |
| 8     | 384.5561                 | 0.4714 | 1.2639 | 17.8304 | 0.6031   | 0.7680   | -0.2154  | x |
|       |                          |        |        |         | -0.5301  | 0.1842   | -0.8277  | y |
|       |                          |        |        |         | -0.5960  | 0.6134   | 0.5182   | z |

**Table S4** Energy levels ( $E$  in  $\text{cm}^{-1}$ ),  $g$ -tensor principal values ( $g_X, g_Y, g_Z$ ), and magnetic axes  $\ell$  for Dy(III) centre 4. Lower-case  $x, y, z$  denote the molecular Cartesian frame; upper-case  $X, Y, Z$  denote the magnetic axes frame.

| Level | $E$ ( $\text{cm}^{-1}$ ) | $g_X$  | $g_Y$  | $g_Z$   | $\ell_X$ | $\ell_Y$ | $\ell_Z$ |   |
|-------|--------------------------|--------|--------|---------|----------|----------|----------|---|
| 1     | 0.0000                   | 0.2246 | 0.6788 | 18.8523 | -0.9917  | 0.0037   | -0.1286  | x |
|       |                          |        |        |         | 0.0537   | 0.9202   | -0.3877  | y |
|       |                          |        |        |         | -0.1169  | 0.3914   | 0.9128   | z |
| 2     | 64.2084                  | 1.4697 | 2.3150 | 15.6634 | 0.8999   | -0.4351  | -0.0293  | x |
|       |                          |        |        |         | 0.0984   | 0.1373   | 0.9856   | y |
|       |                          |        |        |         | -0.4249  | -0.8898  | 0.1664   | z |
| 3     | 112.0278                 | 0.8123 | 2.5048 | 13.4126 | 0.0877   | 0.9587   | -0.2705  | x |
|       |                          |        |        |         | 0.5393   | 0.1826   | 0.8221   | y |
|       |                          |        |        |         | 0.8376   | -0.2179  | -0.5010  | z |
| 4     | 172.0512                 | 1.8078 | 4.3641 | 11.6547 | -0.0809  | 0.4853   | -0.8706  | x |
|       |                          |        |        |         | 0.5274   | 0.7620   | 0.3758   | y |
|       |                          |        |        |         | 0.8458   | -0.4288  | -0.3176  | z |
| 5     | 241.7640                 | 2.4895 | 4.4367 | 11.1259 | -0.4469  | 0.6840   | -0.5766  | x |
|       |                          |        |        |         | -0.8910  | -0.2824  | 0.3556   | y |
|       |                          |        |        |         | 0.0804   | 0.6726   | 0.7356   | z |
| 6     | 304.2819                 | 0.9727 | 2.5583 | 15.3999 | 0.0498   | 0.6670   | -0.7434  | x |
|       |                          |        |        |         | 0.1691   | 0.7279   | 0.6645   | y |
|       |                          |        |        |         | 0.9843   | -0.1588  | -0.0766  | z |
| 7     | 333.3431                 | 1.7829 | 4.6767 | 13.5146 | -0.3294  | -0.1034  | -0.9385  | x |
|       |                          |        |        |         | -0.2612  | 0.9652   | -0.0146  | y |
|       |                          |        |        |         | -0.9073  | -0.2403  | 0.3449   | z |
| 8     | 423.7091                 | 0.1932 | 0.5165 | 18.9094 | -0.4561  | -0.3261  | -0.8280  | x |
|       |                          |        |        |         | 0.8857   | -0.0752  | -0.4582  | y |
|       |                          |        |        |         | -0.0872  | 0.9423   | -0.3231  | z |

**Table S5** Energy levels ( $E$  in  $\text{cm}^{-1}$ ),  $g$ -tensor principal values ( $g_X, g_Y, g_Z$ ), and magnetic axes  $\ell$  for Dy(III) centre 5. Lower-case  $x, y, z$  denote the molecular Cartesian frame; upper-case  $X, Y, Z$  denote the magnetic axes frame.

| Level | $E$ ( $\text{cm}^{-1}$ ) | $g_X$  | $g_Y$  | $g_Z$   | $\ell_X$ | $\ell_Y$ | $\ell_Z$ |   |
|-------|--------------------------|--------|--------|---------|----------|----------|----------|---|
| 1     | 0.0000                   | 0.0006 | 0.0045 | 19.6428 | 0.7739   | -0.3155  | 0.5492   | x |
|       |                          |        |        |         | -0.6311  | -0.3110  | 0.7106   | y |
|       |                          |        |        |         | 0.0533   | 0.8965   | 0.4398   | z |
| 2     | 147.4923                 | 0.1981 | 0.2648 | 16.7278 | 0.1428   | -0.6423  | -0.7530  | x |
|       |                          |        |        |         | -0.7561  | 0.4201   | -0.5018  | y |
|       |                          |        |        |         | 0.6386   | 0.6411   | -0.4256  | z |
| 3     | 270.8987                 | 1.6195 | 2.0257 | 15.6096 | -0.2420  | -0.1813  | -0.9532  | x |
|       |                          |        |        |         | -0.9366  | -0.2128  | 0.2783   | y |
|       |                          |        |        |         | 0.2533   | -0.9601  | 0.1183   | z |
| 4     | 333.4562                 | 1.5166 | 5.8988 | 8.7713  | -0.3239  | -0.3564  | -0.8764  | x |
|       |                          |        |        |         | 0.6952   | -0.7179  | 0.0350   | y |
|       |                          |        |        |         | 0.6417   | 0.5980   | -0.4803  | z |
| 5     | 445.5660                 | 1.3922 | 4.1935 | 8.1047  | 0.8930   | -0.2408  | -0.3801  | x |
|       |                          |        |        |         | 0.3013   | -0.3075  | 0.9026   | y |
|       |                          |        |        |         | -0.3342  | -0.9206  | -0.2021  | z |
| 6     | 499.8369                 | 0.3695 | 3.3657 | 14.2427 | 0.2309   | 0.6899   | -0.6861  | x |
|       |                          |        |        |         | 0.9528   | -0.0173  | 0.3032   | y |
|       |                          |        |        |         | 0.1973   | -0.7237  | -0.6613  | z |
| 7     | 553.1442                 | 0.9772 | 4.1750 | 9.7386  | 0.0210   | 0.9807   | -0.1943  | x |
|       |                          |        |        |         | 0.9707   | 0.0266   | 0.2389   | y |
|       |                          |        |        |         | 0.2395   | -0.1936  | -0.9514  | z |
| 8     | 607.4521                 | 1.2112 | 4.9364 | 15.0897 | -0.9066  | -0.2661  | -0.3275  | x |
|       |                          |        |        |         | 0.0384   | 0.7208   | -0.6920  | y |
|       |                          |        |        |         | -0.4202  | 0.6400   | 0.6433   | z |

**Table S6** Cartesian coordinates (in Å) of the Dy(III) molecular fragment for centre 1.

| Atom | <i>x</i>  | <i>y</i>  | <i>z</i>  | Atom | <i>x</i>  | <i>y</i>  | <i>z</i>  |
|------|-----------|-----------|-----------|------|-----------|-----------|-----------|
| Dy   | 0.000000  | 0.000000  | 0.000000  | H    | 2.370473  | -0.070069 | -4.341756 |
| Ga   | 0.301026  | -2.222745 | -2.552862 | C    | 1.365636  | -0.400928 | -6.051039 |
| N    | -2.173398 | 1.057926  | -0.919286 | H    | 0.944140  | 0.482961  | -6.088112 |
| C    | -3.150469 | 1.209321  | 0.185114  | H    | 0.749197  | -1.072905 | -6.410067 |
| H    | -3.678240 | 2.032909  | 0.034869  | H    | 2.187618  | -0.392555 | -6.585678 |
| H    | -3.777081 | 0.442405  | 0.163650  | O    | 0.589777  | -0.678143 | -3.779799 |
| C    | -2.538500 | 1.277968  | 1.515857  | C    | -1.615513 | -2.507853 | -4.921273 |
| H    | -2.106430 | 2.159589  | 1.640737  | H    | -1.005175 | -2.472638 | -5.701768 |
| H    | -3.236016 | 1.174499  | 2.210498  | H    | -1.887253 | -1.583307 | -4.696881 |
| O    | -1.579224 | 0.248709  | 1.644639  | O    | -0.948580 | -3.102858 | -3.811019 |
| C    | -2.695564 | 0.178901  | -1.969052 | N    | 1.665431  | 2.154570  | 0.948047  |
| H    | -2.260380 | 0.409396  | -2.827596 | O    | 0.420581  | 2.321552  | 0.786095  |
| H    | -3.668044 | 0.340037  | -2.070516 | O    | 2.128173  | 1.018785  | 0.672923  |
| C    | -2.471166 | -1.249766 | -1.682220 | O    | 2.393435  | 3.033686  | 1.396832  |
| H    | -3.039463 | -1.530002 | -0.921237 | Ga   | -0.990192 | -0.921511 | 3.161335  |
| H    | -2.723372 | -1.791244 | -2.470519 | C    | -0.114328 | 1.812893  | 4.079783  |
| O    | -1.105008 | -1.468322 | -1.368071 | H    | 0.761124  | 2.264319  | 3.968562  |
| C    | -1.754425 | 2.328632  | -1.502706 | H    | -0.673641 | 2.035296  | 3.293434  |
| H    | -1.570894 | 2.958402  | -0.761236 | O    | 0.080062  | 0.421630  | 4.136368  |
| H    | -2.518056 | 2.694474  | -2.013930 | N    | -1.981217 | -2.850136 | 2.750990  |
| C    | -0.587116 | 2.325701  | -2.384665 | C    | -1.655409 | -3.773853 | 3.859293  |
| H    | -0.919608 | 2.130334  | -3.307600 | H    | -2.385175 | -3.743293 | 4.526616  |
| C    | 0.146904  | 3.629024  | -2.451007 | H    | -1.611159 | -4.697377 | 3.504168  |
| H    | 0.890680  | 3.554514  | -3.087110 | C    | -0.305357 | -3.442474 | 4.571494  |
| H    | 0.496463  | 3.853499  | -1.563194 | H    | 0.447030  | -3.851714 | 4.077831  |
| H    | -0.465038 | 4.336012  | -2.749546 | H    | -0.311514 | -3.809673 | 5.492478  |
| O    | 0.326261  | 1.260465  | -2.029540 | O    | -0.156050 | -2.086165 | 4.610519  |
| H    | 0.606099  | 0.526858  | -2.614911 | C    | -1.413453 | -3.331648 | 1.498296  |
| N    | 2.371912  | -2.672709 | -3.274429 | H    | -1.507463 | -4.317148 | 1.457320  |
| C    | 3.332295  | -1.977038 | -2.429543 | H    | -1.922860 | -2.947811 | 0.743168  |
| H    | 4.012872  | -1.549626 | -3.009061 | C    | 0.033537  | -2.971089 | 1.351954  |
| H    | 3.797336  | -2.643476 | -1.863685 | H    | 0.333707  | -3.148762 | 0.425116  |
| C    | 2.737781  | -0.942305 | -1.555389 | H    | 0.583275  | -3.515763 | 1.968544  |
| H    | 3.331065  | -0.776097 | -0.780748 | O    | 0.185467  | -1.563455 | 1.662200  |
| H    | 2.641124  | -0.095344 | -2.058808 | C    | -3.416867 | -2.469872 | 2.750990  |
| O    | 1.435462  | -1.380607 | -1.085141 | H    | -3.630736 | -1.984902 | 1.913910  |
| C    | 2.510737  | -4.139531 | -3.200282 | H    | -3.976848 | -3.285943 | 2.786113  |
| H    | 3.469279  | -4.386830 | -3.169062 | C    | -3.729249 | -1.587303 | 3.941245  |
| H    | 2.109484  | -4.557360 | -4.004192 | H    | -3.772899 | -2.180122 | 4.745154  |
| C    | 1.814235  | -4.635098 | -1.967100 | C    | -5.050391 | -0.921433 | 3.816366  |
| H    | 1.823501  | -5.625123 | -1.945637 | H    | -5.205350 | -0.351380 | 4.598812  |
| H    | 2.273627  | -4.298716 | -1.157337 | H    | -5.064663 | -0.372531 | 3.004651  |
| O    | 0.470463  | -4.154447 | -2.008076 | H    | -5.754406 | -1.601695 | 3.763682  |
| C    | 2.342430  | -2.132596 | -4.646148 | O    | -2.687519 | -0.668037 | 4.157832  |
| H    | 1.829061  | -2.744194 | -5.231519 | H    | -2.477442 | -3.096585 | -5.156588 |
| H    | 3.266245  | -2.072621 | -4.999322 | H    | -0.589403 | 2.171957  | 4.968758  |
| C    | 1.690869  | -0.727844 | -4.661758 |      |           |           |           |

**Table S7** Cartesian coordinates (in Å) of the Dy(III) molecular fragment for centre 2.

| Atom | <i>x</i>  | <i>y</i>  | <i>z</i>  | Atom | <i>x</i>  | <i>y</i>  | <i>z</i>  |
|------|-----------|-----------|-----------|------|-----------|-----------|-----------|
| Dy   | 0.000000  | 0.000000  | 0.000000  | H    | -2.912020 | -0.254250 | -3.031640 |
| Ga   | 1.501110  | 3.049960  | 0.601180  | C    | -2.446530 | -1.549080 | -1.681380 |
| Ga   | 1.920530  | -2.469210 | -1.347720 | H    | -1.983900 | -1.936510 | -2.479440 |
| C    | -1.271080 | 4.022940  | 1.471820  | C    | -3.553710 | -2.506310 | -1.599430 |
| O    | 0.095080  | 3.804380  | 1.785970  | H    | -3.212400 | -3.377190 | -1.308690 |
| N    | 3.572000  | 2.600000  | -0.120390 | H    | -3.974280 | -2.597400 | -2.479440 |
| C    | 4.532380  | 3.295670  | 0.724490  | H    | -4.217420 | -2.183220 | -0.953570 |
| H    | 5.212960  | 3.723080  | 0.144980  | O    | -1.439320 | -1.788700 | -0.731130 |
| H    | 4.997420  | 2.629230  | 1.290350  | H    | -0.858450 | -2.326080 | -1.185770 |
| C    | 3.937870  | 4.330400  | 1.598650  | N    | 2.255880  | -4.315390 | -0.149660 |
| H    | 4.531150  | 4.496610  | 2.373290  | C    | 1.709250  | -4.115170 | 1.177180  |
| H    | 3.841210  | 5.177360  | 1.095230  | H    | 2.460360  | -4.021040 | 1.815240  |
| O    | 2.635550  | 3.892100  | 2.068900  | H    | 1.203440  | -4.926440 | 1.432790  |
| C    | 3.710820  | 1.133170  | -0.046240 | C    | 0.835140  | -2.964840 | 1.323520  |
| H    | 4.669370  | 0.885880  | -0.015020 | H    | -0.092020 | -3.226360 | 1.093280  |
| H    | 3.309570  | 0.715350  | -0.850150 | H    | 0.842130  | -2.666800 | 2.265970  |
| C    | 3.014320  | 0.637610  | 1.186940  | O    | 1.242530  | -1.870330 | 0.476690  |
| H    | 3.023590  | -0.352420 | 1.208400  | C    | 3.723890  | -4.518630 | -0.155510 |
| H    | 3.473710  | 0.973990  | 1.996700  | H    | 4.008410  | -4.930120 | -1.010160 |
| O    | 1.670550  | 1.118260  | 1.145960  | H    | 3.990340  | -5.119130 | 0.585960  |
| C    | 3.542520  | 3.140110  | -1.492110 | C    | 4.376270  | -3.148400 | 0.012290  |
| H    | 3.029150  | 2.528510  | -2.077480 | H    | 4.157260  | -2.781690 | 0.905960  |
| H    | 4.466330  | 3.200080  | -1.845280 | H    | 5.360700  | -3.233240 | -0.056000 |
| C    | 2.890960  | 4.544860  | -1.507720 | O    | 3.895560  | -2.278650 | -0.998450 |
| H    | 3.570560  | 5.202640  | -1.187720 | C    | 1.515110  | -5.348220 | -0.867720 |
| C    | 2.565720  | 4.871780  | -2.897000 | H    | 1.424570  | -6.153040 | -0.296000 |
| H    | 2.144230  | 5.755670  | -2.934070 | H    | 2.009150  | -5.606510 | -1.685280 |
| H    | 1.949280  | 4.199800  | -3.256030 | C    | 0.113900  | -4.823360 | -1.252110 |
| H    | 3.387710  | 4.880150  | -3.431640 | H    | -0.464450 | -4.836850 | -0.436490 |
| O    | 1.789870  | 4.594560  | -0.625760 | C    | -0.553700 | -5.667180 | -2.337000 |
| N    | -1.253120 | 0.516630  | -2.147730 | H    | -1.427630 | -5.281550 | -2.557490 |
| C    | -1.623290 | 1.939830  | -2.096990 | H    | -0.674920 | -6.584150 | -2.009190 |
| H    | -2.322380 | 2.079170  | -1.410160 | H    | 0.011880  | -5.677700 | -3.137000 |
| H    | -1.991690 | 2.219450  | -2.973100 | O    | 0.242610  | -3.477330 | -1.691140 |
| C    | -0.415420 | 2.764850  | -1.767240 | C    | 1.968100  | -3.303750 | -4.301890 |
| H    | 0.194910  | 2.800070  | -2.547730 | O    | 2.659230  | -2.846040 | -3.156520 |
| H    | -0.687170 | 3.689400  | -1.542840 | N    | -2.026360 | 0.162700  | 2.029870  |
| O    | 0.251510  | 2.169850  | -0.656980 | O    | -0.956570 | -0.534560 | 2.240610  |
| C    | -0.430100 | 0.128350  | -3.271640 | O    | -2.134770 | 0.797660  | 0.921570  |
| H    | -0.546380 | 0.807620  | -3.983840 | O    | -2.903290 | 0.194920  | 2.904030  |
| H    | -0.777980 | -0.726750 | -3.624810 | H    | -1.769850 | 4.441160  | 2.321060  |
| C    | 1.025230  | -0.031990 | -3.027730 | H    | -1.730360 | 3.092390  | 1.210960  |
| H    | 1.416410  | -0.588270 | -3.747740 | H    | -1.343370 | 4.700090  | 0.646510  |
| H    | 1.461330  | 0.856470  | -3.055050 | H    | 2.655130  | -3.406260 | -5.115760 |
| O    | 1.282290  | -0.638290 | -1.780890 | H    | 1.206820  | -2.599150 | -4.564370 |
| C    | -2.531200 | -0.250530 | -2.118460 | H    | 1.519320  | -4.252210 | -4.092350 |
| H    | -3.169590 | 0.231640  | -1.535040 |      |           |           |           |

**Table S8** Cartesian coordinates (in Å) of the Dy(III) molecular fragment for centre 3.

| Atom | <i>x</i>  | <i>y</i>  | <i>z</i>  | Atom | <i>x</i>  | <i>y</i>  | <i>z</i>  |
|------|-----------|-----------|-----------|------|-----------|-----------|-----------|
| Dy   | 0.000000  | 0.000000  | 0.000000  | C    | 0.014440  | -0.188650 | -3.363310 |
| Ga   | -2.965000 | -0.203960 | 1.743080  | H    | -0.353780 | 0.728410  | -3.435500 |
| Ga   | 2.341720  | -2.407070 | 0.552240  | H    | -0.136670 | -0.647410 | -4.227710 |
| C    | -3.860300 | 2.233250  | 0.063060  | C    | 1.514730  | -0.108860 | -3.092090 |
| H    | -3.469130 | 1.676970  | -0.656940 | H    | 1.916470  | -0.999160 | -3.298920 |
| H    | -3.424200 | 3.121710  | 0.035750  | C    | 2.229670  | 0.968100  | -3.979900 |
| O    | -3.603240 | 1.626950  | 1.309910  | H    | 3.185500  | 0.986530  | -3.763310 |
| N    | -2.629660 | -2.050150 | 2.941140  | H    | 1.837460  | 1.848160  | -3.806240 |
| C    | -3.176290 | -1.849930 | 4.267980  | H    | 2.113870  | 0.738590  | -4.926250 |
| H    | -2.425180 | -1.755800 | 4.906030  | O    | 1.727100  | 0.165350  | -1.734020 |
| H    | -3.682090 | -2.661200 | 4.523590  | H    | 2.399550  | -0.363210 | -1.295000 |
| C    | -4.050390 | -0.699600 | 4.414320  | N    | 4.289030  | -1.772850 | 1.186980  |
| H    | -4.977560 | -0.961120 | 4.184080  | C    | 4.157000  | -0.347400 | 1.709910  |
| H    | -4.043410 | -0.401560 | 5.356770  | H    | 4.019000  | -0.374750 | 2.691380  |
| O    | -3.643000 | 0.394920  | 3.567490  | H    | 4.998740  | 0.141090  | 1.536250  |
| C    | -1.161650 | -2.253390 | 2.935290  | C    | 3.024500  | 0.382640  | 1.075760  |
| H    | -0.877130 | -2.664870 | 2.080640  | H    | 2.833710  | 1.223800  | 1.561610  |
| H    | -0.895190 | -2.853890 | 3.676750  | H    | 3.232860  | 0.597760  | 0.131360  |
| C    | -0.509260 | -0.883160 | 3.103090  | O    | 1.902600  | -0.524470 | 1.159660  |
| H    | -0.728270 | -0.516440 | 3.996760  | C    | 4.509100  | -2.664630 | 2.402600  |
| H    | 0.475170  | -0.968000 | 3.034800  | H    | 4.892930  | -3.529750 | 2.115770  |
| O    | -0.989970 | -0.013410 | 2.092350  | H    | 5.150250  | -2.231910 | 3.021140  |
| C    | -3.370420 | -3.082980 | 2.223080  | C    | 3.207980  | -2.901920 | 3.112850  |
| H    | -3.460970 | -3.887800 | 2.794800  | H    | 3.371020  | -3.528960 | 3.860170  |
| H    | -2.876380 | -3.341270 | 1.405510  | H    | 2.905800  | -2.044110 | 3.503100  |
| C    | -4.771640 | -2.558120 | 1.838690  | O    | 2.130330  | -3.437870 | 2.281620  |
| H    | -5.349980 | -2.571600 | 2.654310  | C    | 5.179730  | -1.921900 | -0.046210 |
| C    | -5.439230 | -3.401930 | 0.753800  | H    | 6.074870  | -1.554930 | 0.162580  |
| H    | -6.313170 | -3.016300 | 0.533310  | H    | 5.287760  | -2.884190 | -0.245230 |
| H    | -5.560460 | -4.318910 | 1.081610  | C    | 4.652720  | -1.234080 | -1.265730 |
| H    | -4.873660 | -3.412460 | -0.046210 | H    | 4.745150  | -0.240050 | -1.209140 |
| O    | -4.642920 | -1.212090 | 1.399660  | C    | 5.203280  | -1.806610 | -2.619890 |
| N    | -0.688440 | -0.901140 | -2.315490 | H    | 4.837770  | -1.287350 | -3.367210 |
| C    | -2.177530 | -0.628350 | -2.444280 | H    | 4.934680  | -2.745090 | -2.711590 |
| H    | -2.322190 | 0.337800  | -2.606230 | H    | 6.181970  | -1.744790 | -2.627690 |
| H    | -2.535910 | -1.124590 | -3.222820 | O    | 3.362260  | -1.659630 | -0.974990 |
| C    | -2.917430 | -1.038500 | -1.211090 | C    | 2.815760  | -4.667530 | -1.402310 |
| H    | -3.829650 | -0.655280 | -1.224750 | H    | 3.789780  | -4.671750 | -1.579880 |
| H    | -2.995570 | -2.025280 | -1.181820 | H    | 2.389390  | -4.036520 | -2.032560 |
| O    | -2.226300 | -0.580800 | -0.065720 | O    | 2.579210  | -4.250940 | -0.083280 |
| C    | -0.385060 | -2.360340 | -2.362320 | N    | 0.149640  | 2.811180  | -0.555480 |
| H    | 0.472210  | -2.493340 | -2.838420 | O    | 0.823840  | 2.312120  | 0.347950  |
| H    | -1.092560 | -2.815820 | -2.885250 | O    | -0.731620 | 2.056910  | -1.123290 |
| C    | -0.291670 | -3.005160 | -1.010120 | O    | 0.274330  | 3.967950  | -0.949630 |
| H    | -1.200320 | -3.116400 | -0.633530 | H    | 2.410850  | -5.649420 | -1.532070 |
| H    | 0.117700  | -3.902370 | -1.097920 | H    | -4.917270 | 2.331190  | -0.071590 |
| O    | 0.490010  | -2.209670 | -0.137910 |      |           |           |           |

**Table S9** Cartesian coordinates (in Å) of the Dy(III) molecular fragment for centre 4.

| Atom | <i>x</i>  | <i>y</i>  | <i>z</i>  | Atom | <i>x</i>  | <i>y</i>  | <i>z</i>  |
|------|-----------|-----------|-----------|------|-----------|-----------|-----------|
| Dy   | 0.000000  | 0.000000  | 0.000000  | C    | -0.239520 | -2.441860 | -2.267400 |
| Ga   | 0.328040  | 3.254530  | -1.095290 | H    | 0.179280  | -3.045970 | -2.928870 |
| Ga   | 2.441630  | -1.416090 | 1.893030  | H    | -1.105620 | -2.150240 | -2.647890 |
| C    | -2.305350 | 2.656440  | -2.657640 | C    | -0.537120 | -3.248830 | -1.055680 |
| H    | -3.214000 | 2.545200  | -2.281050 | H    | 0.192360  | -3.928370 | -0.999090 |
| H    | -1.895980 | 1.759230  | -2.745450 | C    | -1.823270 | -4.035410 | -1.151290 |
| O    | -1.523670 | 3.451930  | -1.785440 | H    | -1.944840 | -4.562050 | -0.333720 |
| N    | 2.275350  | 3.888750  | -0.460550 | H    | -1.783980 | -4.635470 | -1.923980 |
| C    | 2.143320  | 5.314210  | 0.062380  | H    | -2.578310 | -3.417350 | -1.256660 |
| H    | 2.005320  | 5.286860  | 1.043850  | O    | -0.381940 | -2.390270 | 0.150190  |
| H    | 2.985060  | 5.802690  | -0.111280 | H    | 0.045250  | -2.629400 | 0.998970  |
| C    | 1.010820  | 6.044250  | -0.571770 | N    | 1.977590  | -1.904720 | 4.011680  |
| H    | 0.820030  | 6.885410  | -0.085910 | C    | 0.652730  | -1.302910 | 4.390220  |
| H    | 1.219180  | 6.259360  | -1.516170 | H    | 0.135280  | -1.959870 | 4.919010  |
| O    | -0.111080 | 5.137140  | -0.487870 | H    | 0.806640  | -0.508700 | 4.959990  |
| C    | 2.495420  | 2.996970  | 0.755070  | C    | -0.125000 | -0.910690 | 3.211680  |
| H    | 2.879250  | 2.131860  | 0.468240  | H    | -0.642640 | -1.691900 | 2.895580  |
| H    | 3.136570  | 3.429700  | 1.373610  | H    | -0.772170 | -0.209870 | 3.475090  |
| C    | 1.194300  | 2.759690  | 1.465320  | O    | 0.666040  | -0.419220 | 2.128740  |
| H    | 1.357340  | 2.132650  | 2.212640  | C    | 2.990270  | -1.276830 | 4.819500  |
| H    | 0.892120  | 3.617500  | 1.855570  | H    | 3.785890  | -1.864050 | 4.868280  |
| O    | 0.116650  | 2.223730  | 0.634090  | H    | 2.645760  | -1.145110 | 5.738530  |
| C    | 3.166050  | 3.739700  | -1.693730 | C    | 3.406060  | 0.121800  | 4.208760  |
| H    | 4.061190  | 4.106680  | -1.484950 | H    | 2.666620  | 0.773170  | 4.284860  |
| H    | 3.274080  | 2.777410  | -1.892760 | H    | 4.203550  | 0.484200  | 4.669250  |
| C    | 2.639040  | 4.427520  | -2.913260 | O    | 3.697680  | -0.173530 | 2.819480  |
| H    | 2.731470  | 5.421550  | -2.856670 | C    | 1.968570  | -3.454860 | 3.896560  |
| C    | 3.189600  | 3.854990  | -4.267410 | H    | 2.900080  | -3.778120 | 3.818510  |
| H    | 2.824090  | 4.374250  | -5.014740 | H    | 1.582350  | -3.836620 | 4.723890  |
| H    | 2.921000  | 2.916510  | -4.359120 | C    | 1.209720  | -3.929050 | 2.762890  |
| H    | 4.168290  | 3.916820  | -4.275220 | H    | 0.232460  | -3.847980 | 2.963870  |
| O    | 1.348580  | 4.001980  | -2.622520 | C    | 1.566110  | -5.394040 | 2.587280  |
| N    | 0.614630  | -1.250110 | -2.162030 | H    | 1.083760  | -5.756170 | 1.814590  |
| C    | 0.243310  | -0.391570 | -3.264480 | H    | 1.310440  | -5.889960 | 3.393140  |
| H    | -0.743480 | -0.345560 | -3.334720 | H    | 2.530090  | -5.478810 | 2.440940  |
| H    | 0.596480  | -0.765240 | -4.111310 | O    | 1.509600  | -3.147780 | 1.660440  |
| C    | 0.802080  | 0.994080  | -3.049840 | C    | 4.525050  | -3.360780 | 0.663360  |
| H    | 1.776100  | 0.989850  | -3.227400 | H    | 4.647730  | -3.103570 | -0.284940 |
| H    | 0.375710  | 1.625080  | -3.680090 | H    | 3.767430  | -3.996080 | 0.710190  |
| O    | 0.565530  | 1.410670  | -1.730810 | O    | 4.212480  | -2.208720 | 1.422390  |
| C    | 2.084980  | -1.552240 | -2.097640 | N    | -2.850930 | -0.227890 | 0.070190  |
| H    | 2.198670  | -2.510110 | -1.869340 | O    | -2.196810 | -0.014110 | 1.098490  |
| H    | 2.472730  | -1.412510 | -2.997160 | O    | -2.194730 | -0.183460 | -1.030310 |
| C    | 2.850600  | -0.754990 | -1.135680 | O    | -4.044780 | -0.413970 | 0.089700  |
| H    | 3.732360  | -1.176560 | -0.989340 | H    | 5.416980  | -3.807900 | 1.049940  |
| H    | 3.002850  | 0.149920  | -1.508370 | H    | -2.355430 | 3.136800  | -3.612440 |
| O    | 2.183500  | -0.641120 | 0.093600  |      |           |           |           |

**Table S10** Cartesian coordinates (in Å) of the Dy(III) molecular fragment for centre 5.

| Atom | <i>x</i>  | <i>y</i>  | <i>z</i>  | Atom | <i>x</i>  | <i>y</i>  | <i>z</i>  |
|------|-----------|-----------|-----------|------|-----------|-----------|-----------|
| Dy   | 0.000000  | 0.000000  | 0.000000  | C    | 2.016800  | -2.310460 | -1.341140 |
| Ga   | -3.373310 | -0.640580 | -0.244160 | H    | 1.653850  | -2.255100 | -2.260180 |
| Ga   | 1.640480  | 0.298840  | 2.950990  | H    | 2.534590  | -3.151360 | -1.282610 |
| C    | -2.964340 | 0.020510  | -3.272870 | C    | 2.953640  | -1.195940 | -1.163580 |
| H    | -2.082580 | -0.401050 | -3.126530 | H    | 3.604140  | -1.578680 | -0.506010 |
| H    | -2.812090 | 0.925420  | -3.645550 | C    | 3.829360  | -0.790590 | -2.244570 |
| O    | -3.631440 | 0.134390  | -2.043590 | H    | 4.404820  | -0.056540 | -1.944080 |
| N    | -3.837350 | -1.129220 | 1.874490  | H    | 3.290160  | -0.491340 | -3.007500 |
| C    | -5.162210 | -0.527410 | 2.253030  | H    | 4.385900  | -1.550890 | -2.517740 |
| H    | -5.679660 | -1.184360 | 2.781820  | O    | 2.402740  | -0.097150 | -0.420160 |
| H    | -5.008300 | 0.266810  | 2.822800  | H    | 2.806940  | 0.111230  | 0.383750  |
| C    | -5.939940 | -0.135190 | 1.074490  | N    | 2.631500  | 2.227470  | 3.361340  |
| H    | -6.457580 | -0.916400 | 0.758390  | C    | 2.305690  | 3.151180  | 2.253030  |
| H    | -6.587110 | 0.565640  | 1.337900  | H    | 3.035460  | 3.120620  | 1.585710  |
| O    | -5.148900 | 0.356290  | -0.008450 | H    | 2.261440  | 4.074710  | 2.608160  |
| C    | -2.824670 | -0.501330 | 2.682310  | C    | 0.955640  | 2.819810  | 1.540830  |
| H    | -2.029050 | -1.088540 | 2.731090  | H    | 0.203250  | 3.229050  | 2.034500  |
| H    | -3.169190 | -0.369610 | 3.601340  | H    | 0.961800  | 3.187000  | 0.619850  |
| C    | -2.408880 | 0.897310  | 2.071570  | O    | 0.806330  | 1.463500  | 1.501810  |
| H    | -3.148320 | 1.548670  | 2.147670  | C    | 2.063740  | 2.708980  | 4.614030  |
| H    | -1.611390 | 1.259700  | 2.532060  | H    | 2.157750  | 3.694480  | 4.655010  |
| O    | -2.117260 | 0.601970  | 0.682290  | H    | 2.573140  | 2.325140  | 5.369160  |
| C    | -3.846380 | -2.679360 | 1.759370  | C    | 0.616750  | 2.348420  | 4.760370  |
| H    | -2.914860 | -3.002620 | 1.681320  | H    | 0.316580  | 2.526090  | 5.687210  |
| H    | -4.232590 | -3.061120 | 2.586700  | H    | 0.067010  | 2.893090  | 4.143780  |
| C    | -4.605220 | -3.153540 | 0.625700  | O    | 0.464820  | 0.940790  | 4.450130  |
| H    | -5.582480 | -3.072470 | 0.826680  | C    | 4.067150  | 1.847200  | 3.361340  |
| C    | -4.248830 | -4.618530 | 0.450090  | H    | 4.281020  | 1.362230  | 4.198420  |
| H    | -4.731180 | -4.980670 | -0.322600 | H    | 4.627130  | 2.663270  | 3.326220  |
| H    | -4.504500 | -5.114460 | 1.255950  | C    | 4.379530  | 0.964630  | 2.171080  |
| H    | -3.284850 | -4.703310 | 0.303750  | H    | 4.423180  | 1.557450  | 1.367170  |
| O    | -4.305340 | -2.372280 | -0.476750 | C    | 5.700670  | 0.298760  | 2.295960  |
| N    | 0.920710  | -2.413480 | -0.447480 | H    | 5.855630  | -0.271290 | 1.513520  |
| C    | -0.103940 | -3.225610 | -1.001630 | H    | 5.714950  | -0.250140 | 3.107680  |
| H    | -0.370920 | -3.886150 | -0.312840 | H    | 6.404690  | 0.979030  | 2.348650  |
| H    | 0.285240  | -3.732440 | -1.756760 | O    | 3.337800  | 0.045370  | 1.954500  |
| C    | -1.289890 | -2.585270 | -1.473830 | N    | 0.028230  | 1.591480  | -2.402620 |
| H    | -1.167220 | -2.328070 | -2.422130 | O    | 0.212670  | 0.333780  | -2.422130 |
| H    | -2.047510 | -3.220580 | -1.427000 | O    | -0.122870 | 2.117430  | -1.282610 |
| O    | -1.602460 | -1.433220 | -0.714800 | O    | -0.016110 | 2.250890  | -3.438720 |
| C    | 1.414250  | -2.926560 | 0.816920  | C    | 3.188780  | -1.900640 | 4.596470  |
| H    | 2.379860  | -2.714820 | 0.877410  | H    | 2.756710  | -2.782260 | 4.471590  |
| H    | 1.330680  | -3.913200 | 0.801310  | H    | 3.886300  | -1.797170 | 3.901830  |
| C    | 0.764610  | -2.435560 | 2.032550  | O    | 2.229510  | -0.871380 | 4.467690  |
| H    | -0.110840 | -2.886990 | 2.143770  | H    | -3.555070 | -0.567790 | -3.943560 |
| H    | 1.323920  | -2.657970 | 2.818890  | H    | 3.624710  | -1.839350 | 5.571720  |
| O    | 0.570220  | -1.044300 | 1.975960  |      |           |           |           |



## 2 Supplementary Note 2: Toroidal and Magnetic Spectrum

To highlight the fact that most states are endowed with both toroidal and magnetic moment properties, we report in Figure S1 a graphical table representing the toroidal moments and magnetic moments for the six lowest Kramers Doublets as calculated via our ab initio parameterised model.

|   | $E \text{ (cm}^{-1}\text{)}$ | $\tau/a_0\mu_B$                                                 | $ \tau /a_0\mu_B$ | $\mu/\mu_B$                                                      | $ \mu /\mu_B$ | Figure |    | $E \text{ (cm}^{-1}\text{)}$ | $\tau/a_0\mu_B$                                                 | $ \tau /a_0\mu_B$ | $\mu/\mu_B$                                                     | $ \mu /\mu_B$ | Figure |
|---|------------------------------|-----------------------------------------------------------------|-------------------|------------------------------------------------------------------|---------------|--------|----|------------------------------|-----------------------------------------------------------------|-------------------|-----------------------------------------------------------------|---------------|--------|
| 1 | 0                            | $\begin{pmatrix} 167.757 \\ -97.5775 \\ -2572.3 \end{pmatrix}$  | 2579.61           | $\begin{pmatrix} 0 \\ 0 \\ 0 \end{pmatrix}$                      | 0             |        | 7  | 0.510036                     | $\begin{pmatrix} -632.091 \\ -297.137 \\ 458.263 \end{pmatrix}$ | 835.364           | $\begin{pmatrix} 70.5043 \\ -12.5991 \\ 7.20025 \end{pmatrix}$  | 71.9822       |        |
| 2 | 0                            | $\begin{pmatrix} -167.757 \\ 97.5775 \\ 2572.3 \end{pmatrix}$   | 2579.61           | $\begin{pmatrix} 0 \\ 0 \\ 0 \end{pmatrix}$                      | 0             |        | 8  | 0.510036                     | $\begin{pmatrix} 632.091 \\ 297.137 \\ -458.263 \end{pmatrix}$  | 835.364           | $\begin{pmatrix} -70.5043 \\ 12.5991 \\ -7.20025 \end{pmatrix}$ | 71.9822       |        |
| 3 | 0.259241                     | $\begin{pmatrix} 0 \\ 0 \\ 0 \end{pmatrix}$                     | 0                 | $\begin{pmatrix} 77.5757 \\ 6.59177 \\ 29.6229 \end{pmatrix}$    | 83.3004       |        | 9  | 0.76083                      | $\begin{pmatrix} 0 \\ 0 \\ 0 \end{pmatrix}$                     | 0                 | $\begin{pmatrix} -63.4328 \\ 31.7899 \\ 15.2224 \end{pmatrix}$  | 72.5675       |        |
| 4 | 0.259241                     | $\begin{pmatrix} 0 \\ 0 \\ 0 \end{pmatrix}$                     | 0                 | $\begin{pmatrix} -77.5757 \\ -6.59177 \\ -29.6229 \end{pmatrix}$ | 83.3004       |        | 10 | 0.76083                      | $\begin{pmatrix} 0 \\ 0 \\ 0 \end{pmatrix}$                     | 0                 | $\begin{pmatrix} 63.4328 \\ -31.7899 \\ -15.2224 \end{pmatrix}$ | 72.5675       |        |
| 5 | 0.510035                     | $\begin{pmatrix} 632.091 \\ 297.137 \\ -458.263 \end{pmatrix}$  | 835.364           | $\begin{pmatrix} 70.5043 \\ -12.5991 \\ 7.20025 \end{pmatrix}$   | 71.9822       |        | 11 | 0.798731                     | $\begin{pmatrix} -70.232 \\ 521.014 \\ 1640.13 \end{pmatrix}$   | 1722.33           | $\begin{pmatrix} 27.32 \\ 41.1455 \\ 5.68247 \end{pmatrix}$     | 49.7154       |        |
| 6 | 0.510035                     | $\begin{pmatrix} -632.091 \\ -297.137 \\ 458.263 \end{pmatrix}$ | 835.364           | $\begin{pmatrix} -70.5043 \\ 12.5991 \\ -7.20025 \end{pmatrix}$  | 71.9822       |        | 12 | 0.798731                     | $\begin{pmatrix} 70.232 \\ -521.014 \\ -1640.13 \end{pmatrix}$  | 1722.33           | $\begin{pmatrix} -27.32 \\ -41.1455 \\ -5.68247 \end{pmatrix}$  | 49.7154       |        |

**Fig. S1** The six lowest energy Kramers doublets of  $\text{Fe}_{10}\text{Dy}_{10}$  computed using our parameter free theoretical model. We report the energy  $E$ , three-dimensional toroidal moment  $\tau$ , its magnitude  $|\tau|$ , the three-dimensional magnetic moment  $\mu$  and its magnitude  $|\mu|$  for each state. The  $\text{Dy}^{\text{III}}$  magnetic moment orientations for each state are shown as orange arrows at the site of each  $\text{Dy}^{\text{III}}$  atom (blue spheres) with the toroidal moment and magnetic moment depicted as green and purple arrows, respectively. Note that most states support both toroidal and magnetic moments simultaneously, however the largest toroidal and magnetic moments appear in the ground and first excited states, respectively, as pure quantities.

### 3 Supplementary Note 3: Synthesis

[Fe<sub>10</sub>Dy<sub>10</sub>(Me-tea)<sub>10</sub>(Me-teaH)<sub>10</sub>(NO<sub>3</sub>)<sub>10</sub>] (see Figure S2) can be synthesised after a procedure some of us published previously [3], and the crystal structure was deposited at the Cambridge Crystallographic Data Centre (CCDC) with deposition number 885249. However, we found that using the following adapted procedure results in higher yields and better crystallinity of the product.

Fe(NO<sub>3</sub>)<sub>3</sub> · 9H<sub>2</sub>O (0.25 mmol) and Dy(NO<sub>3</sub>)<sub>3</sub> · 6H<sub>2</sub>O (0.25 mmol) were dissolved in 5 ml MeOH. A solution of Me-teaH<sub>3</sub> (1 mmol) and Et<sub>3</sub>N (0.7 mmol) in 10 ml MeCN was added dropwise under stirring. After 10 minutes additional 80 μl of Et<sub>3</sub>N (0.6 mmol) were added and the solution stirred for another 10 minutes. This resulted in a clear light brown solution which was left undisturbed for crystallisation. After two weeks the product was isolated as colourless block shaped crystals in a yield of 77% (based on Dy).

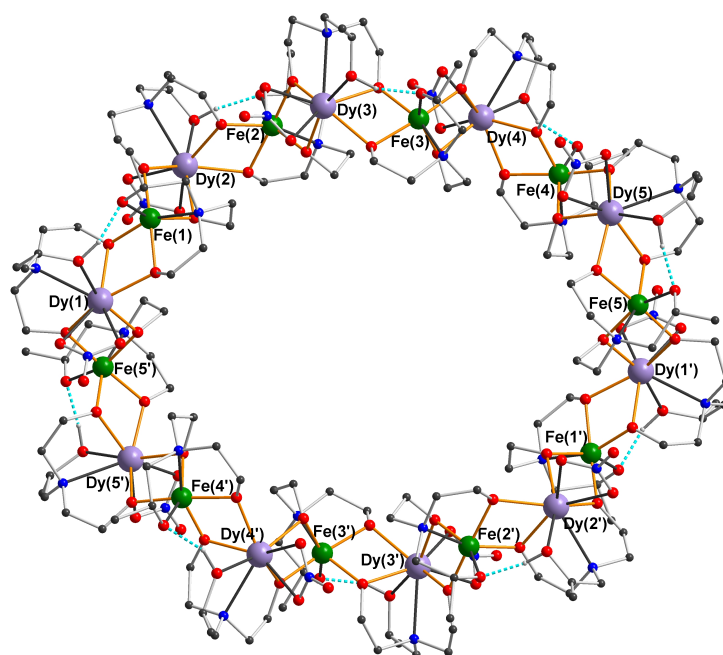

**Fig. S2** Molecular structure of Fe<sub>10</sub>Dy<sub>10</sub>.

## 4 Supplementary Note 4: AC SQUID Magnetometry

A randomly oriented powder sample of  $\text{Fe}_{10}\text{Dy}_{10}$  was immobilised in eicosane and the sample tested for slow relaxation of magnetisation using AC susceptometry. The compound shows slow relaxation with maxima in the out-of-phase component of the susceptibility below 1.8 K and above 1500 Hz and thus outside of our measurement window (see Figure S3).

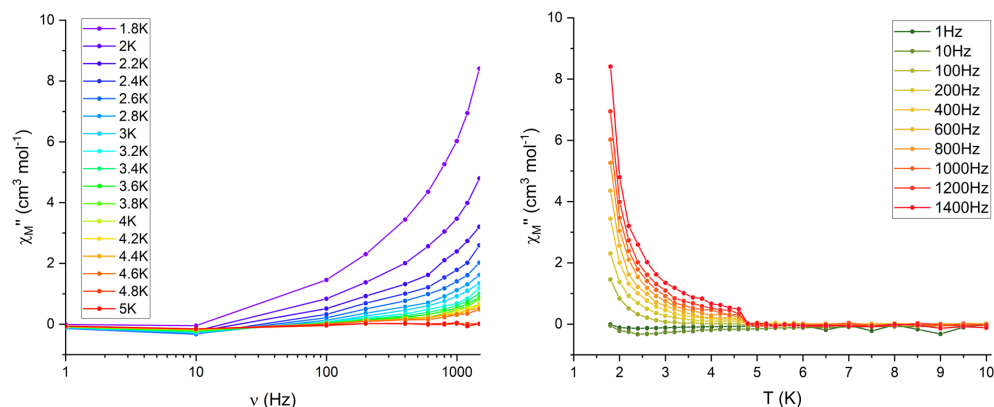

**Fig. S3** Frequency dependence (left) and temperature dependence (right) of the out-of-phase component of the susceptibility indicating slow relaxation of magnetisation at low temperatures.

## 5 Supplementary Note 5: MicroSQUID

In order to assess the magnetic behavior below 1.8 K microSQUID measurements were conducted on a single crystal of  $\text{Fe}_{10}\text{Dy}_{10}$  (see Figure S4).

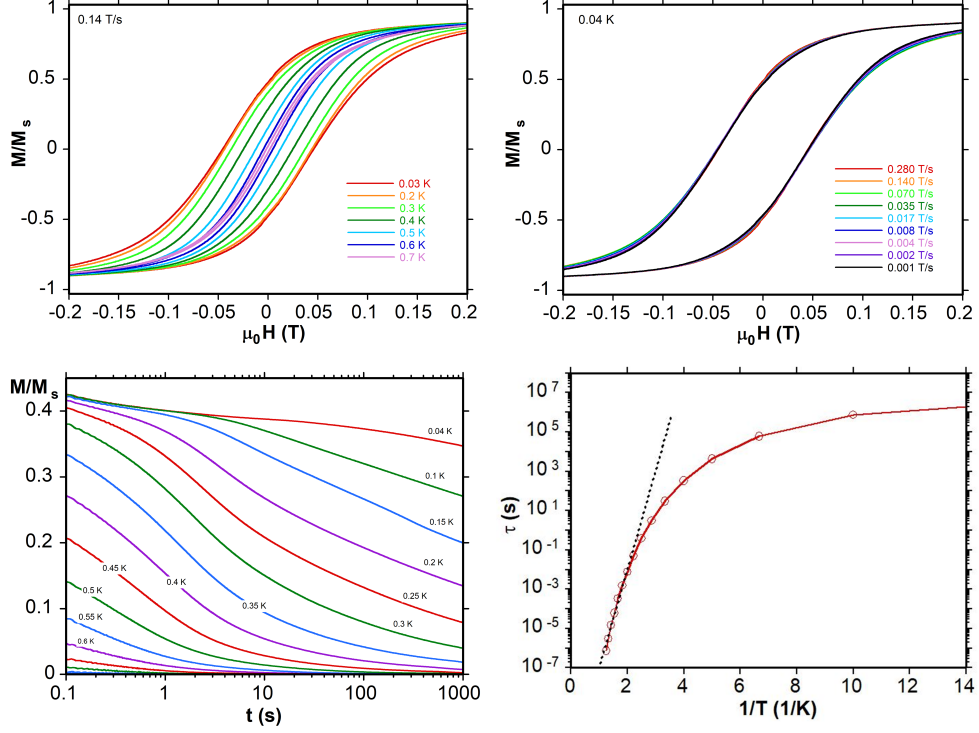

**Fig. S4** Single crystal microSQUID data. Top left: Temperature dependence between 0.03 and 0.7 K at a field sweep rate of 0.14 T/s. Top right: Sweep rate dependence at 0.04 K. Bottom left: Magnetisation decay between 0.04 and 0.6 K. Bottom right: Relaxation times extracted from magnetisation decay plotted against  $1/T$ . The linear fit results in an energy barrier  $U = 11.5$  K and  $\tau_0 = 8 \cdot 10^{-13}$  s.

While these measurements are not directly relevant to assess the toroidal character of the low-energy states, the measured magnetic hysteresis with a coercive field of  $\sim 50$  mT observed here in Figure S4 is consistent with what was obtained in our single-crystal simulations of the low-temperature static equilibrium magnetisation reported in Figure 5a of the main text. In our simulations in fact, the level crossings between the non-magnetic zero-temperature ground state (i.e. the maximally toroidal s-wave Ising vortex state), and a magnetic excitation, occurs for fields between 6 mT and 40 mT, according to the specific orientation of the external magnetic field. The fact that the coercive field observed in the experiment is somewhat larger is not surprising for this kind of systems. In fact, as shown previously by some of us for the  $\text{CrDy}_6$  wheels [4, 5], magnetic relaxation in systems with a toroidal ground state formally resulting from

the ferrotoroidic coupling of an upper and a lower toroidal moiety (imagine here the 5 Dy ions living above (below) the median plane as the upper (lower) toroidal moiety), typically involve a dense cascade of excited magnetic states with very large magnetic moments giving rise to a dense succession of level crossings mediating the population transfer between the maximally magnetic states, stable at large values of the sweeping magnetic field. The dense character of the magnetic excitations (see also Figure 2c), some of which very low-lying in energy, can thus explain the apparent absence in the single-crystal dynamical magnetization profile of any signature of the non-magnetic zero-field ground state with maximal toroidal moment. This picture is also consistent with the smooth character of the observed dynamical magnetic hysteresis in Figure S4 when compared to the steep nature of the simulated low-temperature equilibrium magnetization in Figure 5a, and with the somewhat larger coercive fields observed on average in the dynamical experiments.

## References

- [1] Van den Heuvel, W., Calvello, S. & Soncini, A. Configuration-averaged 4f orbitals in ab initio calculations of low-lying crystal field levels in lanthanide(III) complexes. *Physical Chemistry Chemical Physics* **18**, 15807–15814 (2016).
- [2] Calvello, S., Piccardo, M., Rao, S. V. & Soncini, A. CERES: An ab initio code dedicated to the calculation of the electronic structure and magnetic properties of lanthanide complexes. *Journal of Computational Chemistry* **39**, 328–337 (2018).
- [3] Baniodeh, A. *et al.* Unraveling the influence of lanthanide ions on intra- and inter-molecular electronic processes in Fe<sub>10</sub>Ln<sub>10</sub> nano-toruses. *Advanced Functional Materials* **24**, 6280–6290 (2014).
- [4] Vignesh, K. R. *et al.* Ferrotoroidic ground state in a heterometallic {Cr<sup>III</sup>Dy<sub>6</sub><sup>III</sup>} complex displaying slow magnetic relaxation. *Nature Communications* **8**, 1–12 (2017).
- [5] Ashtree, J. M. *et al.* Tuning the ferrotoroidic coupling and magnetic hysteresis in double-triangle complexes {Dy<sub>3</sub>M<sup>III</sup>Dy<sub>3</sub>} via the M<sup>III</sup>-linker. *European Journal of Inorganic Chemistry* **2021**, 435–444 (2021).
